# Supplementary material for: Compactness and non-compactness theorems of the fourth- and sixth-order constant $Q$-curvature problems
Source: arXiv:2502.14237 ancillary file (2025-09-19)
Supplement: Supplementary file 1 [file Lemma_B.13.pdf]

```

In[*]:= (* Integrals and coefficients *)
Int[i_, j_] := Integrate[t^i / (1 + t^2)^j, {t, 0, Infinity}]
Int2[i_, j_] := Integrate[(1 - t^2) t^i / (1 + t^2)^j, {t, 0, Infinity}]
c1[n_, k_, m_] := (k + m) (n^3 - (k + m + 2) n^2 + (6 (k + m) - 4) n - 4 (k + m) + 8)
c2[n_, k_, m_] := 2 (n - 1) (k + m) (n + k + m - 2) k m;
A[n_, k_, q_] :=
  (k - 2 q - 1) (2 - (n - 2) / (n - 1) * (n + k - 2 q - 1)) - (q + 1) (n + 2 k - 2 q - 4)
kappa[n_, s_] := (n - 2) / (n - 1) * s (s - 1) (n + s - 1) (n + s - 2)

In[*]:= (* Case 3: Estimate of  $I_{\epsilon}$  with  $H = \hat{H}$  *)
(** The matrix and vectors **)
(***) The matrix  $A$  in Section 4 (***)
linearizedMatrix[n_, k_, s_] := Module[{M, j}, M = ConstantArray[0, {s + 4, s + 3}];
  M[[1, 1]] = 4 * (n - 2) * n * (n + 2) * (k - 2 * s - 1);
  M[[2, 1]] = 4 * (n - 2) * n * (k - 2 * s) * (k - 2 * s - 1);
  For[j = 2, j ≤ s + 3, j++,
    M[[j - 1, j]] = -8 * (j - 1) * (n + 2 - j) * (n^2 - 2 * (j - 2) * n + 2 * j * (j - 3));
    M[[j, j]] = 4 * (n - 2 * j) * (n + 2 - 2 * j) * (n + 4 - 2 * j) * (k - 2 * s + j - 2);
    M[[j + 1, j]] = 4 * (n - 2 * j) * (n + 2 - 2 * j) * (k - 2 * s + j - 1) * (k - 2 * s + j - 2);];
  M]

(***) The vector  $b$  in Section 4 (***)
linearizedVector[n_, k_, s_] := Module[{b, i}, b = ConstantArray[0, s + 4];
  b[[3]] = (-1)^s * (n^2 - 4 * n + 8);
  b[[4]] = (-1)^(s + 1) * (s * (n^2 - 4 * n + 8) - (k + 2) * (n - 6));
  b[[s + 4]] = (k + 2) * (n - 6) - s * (2 * k - 2 * s + n - 2);
  If[s - 1 > 0, For[i = 5, i ≤ s + 3, i++,
    b[[i]] = (-1)^(s + 3 - i) * ((n^2 - 4 * n + 8) * Binomial[s, i - 3] + s * (2 * k - 2 * s + n - 2) *
      Binomial[s - 1, i - 5] - (k + 2) * (n - 6) * Binomial[s, i - 4]);];
  b]

(***) The vector  $\gamma$  in Section 4 (***)
LAnswer[n_, k_, s_] :=
  Module[{}, LinearSolve[linearizedMatrix[n, k, s], linearizedVector[n, k, s]]]

(***) The vector  $b'$  in Section 4 (***)
linearizedVectorPrime[n_, k_, s_] :=
  Module[{bPrime, i}, bPrime = ConstantArray[0, s + 4];
  bPrime[[3]] = (-1)^s * n * (n^2 - 4 * n + 8);
  bPrime[[4]] = (-1)^(s + 1) * (s * n * (n^2 - 4 * n + 8) - (k * (n - 2) * (n - 6) - 8 (n - 1)));
  bPrime[[s + 4]] = (k * (n - 2) * (n - 6) - 8 (n - 1)) - (n - 4) * s * (2 * k - 2 * s + n - 2);
  If[s - 1 > 0, For[i = 5, i ≤ s + 3, i++,
    bPrime[[i]] = (-1)^(s + 3 - i) * (n * (n^2 - 4 * n + 8) * Binomial[s, i - 3] +
      (n - 4) * s * (2 * k - 2 * s + n - 2) * Binomial[s - 1, i - 5] -
      (k * (n - 2) * (n - 6) - 8 (n - 1)) * Binomial[s, i - 4]);];
  bPrime]

```

```

(** Definition of the matrices **)
MathH1[n_, s_] := Module[{d, Msize, q, qPrime, k, m, lambdaq, lambdaqPrime, M},
  d = Floor[(n - 4) / 2];
  Msize = Floor[(d - s) / 2];
  M = ConstantArray[0, {Msize, Msize}];
  For[q = 1, q ≤ Msize, q++,
    For[qPrime = 1, qPrime ≤ Msize, qPrime++,
      k = 2 q + s;
      m = 2 qPrime + s;
      lambdaq = A[n, 2 q + s, q];
      lambdaqPrime = A[n, 2 qPrime + s, qPrime];
      If[k + m < n - 4, M[[q, qPrime]] =
        (n - 4)^2 * kappa[n, s] / (4 (n - 1) * (n - 2) * (n - k - m - 4)) * Int[n + k + m - 3, n - 2]
        ((8 (n - 1) * (n - 3) * (k + m) * lambdaq * lambdaqPrime) / ((n - 2) * (n + k + m - 4)) +
        (4 (n - 3) * (k + m) * (s - 1) * (n + s - 1) * k * m) / (n + k + m - 4) -
        ((n - 3) * n^2 * (n - 4) * (k + m) * kappa[n, s]) /
        (2 (n - 1) * (n - 2) * (n + k + m - 4)) + (1 / 8 * c1[n, k, m] *
        (2 (lambdaq + lambdaqPrime) + (n + k + m - 2) (k + m)) - c2[n, k, m])),
      M[[q, qPrime]] = 10^10 (n - 4)^2 * kappa[n, s] / (8 (n - 1) * (n - 2) * (n - 3)) *
        ((8 (n - 1) * (n - 3) * (k + m) * lambdaq * lambdaqPrime) / ((n - 2) * (n + k + m - 4)) +
        (4 (n - 3) * (k + m) * (s - 1) * (n + s - 1) * k * m) / (n + k + m - 4) -
        ((n - 3) * n^2 * (n - 4) * (k + m) * kappa[n, s]) /
        (2 (n - 1) * (n - 2) * (n + k + m - 4)) + (1 / 8 * c1[n, k, m] *
        (2 (lambdaq + lambdaqPrime) + (n + k + m - 2) (k + m)) - c2[n, k, m]))];];];
  M] (* // MatrixForm *)

MathH2[n_, s_] := Module[{d, Msize, q, qPrime, k, m, M, MSymm},
  d = Floor[(n - 4) / 2];
  Msize = Floor[(d - s) / 2];
  M = ConstantArray[0, {Msize, Msize}];
  MSymm = ConstantArray[0, {Msize, Msize}];
  For[q = 1, q ≤ Msize, q++,
    For[qPrime = 1, qPrime ≤ Msize, qPrime++,
      k = 2 q + s;
      m = 2 qPrime + s;
      If[k + m < n - 4, M[[q, qPrime]] = -1 / 2 * ((n - 4) * kappa[n, s] / (2 (n - 1)))^2 *
        Sum[linearizedVector[n, m - 2, qPrime - 1][[i]] * LAnswer[n, k - 2, q - 1][[j]] *
        (((n - 2 s - 2 i - 2 j + 6) * (n - 2 j)) / (n + 3 - i - j) - (n + 4 - 4 j - 2 s)) * Int[n - 1 +
        2 s, n + 3 - i - j], {i, 1, qPrime + 3}, {j, 1, q + 2}], M[[q, qPrime]] = 0];];];
  For[q = 1, q ≤ Msize, q++,
    For[qPrime = 1, qPrime ≤ Msize, qPrime++,
      k = 2 q + s;
      m = 2 qPrime + s;
      If[k + m < n - 4, MSymm[[q, qPrime]] = (M[[q, qPrime]] + M[[qPrime, q]]) / 2,
      MSymm[[q, qPrime]] = 10^10 (M[[q, qPrime]] + M[[qPrime, q]]) / 2];];];
  MSymm] (* // MatrixForm *)

MathH3[n_, s_] := Module[{d, Msize, q, qPrime, k, m, M, MSymm},
  d = Floor[(n - 4) / 2];

```

```

Msize = Floor[(d - s) / 2];
M = ConstantArray[0, {Msize, Msize}];
MSymm = ConstantArray[0, {Msize, Msize}];
For[q = 1, q ≤ Msize, q++,
  For[qPrime = 1, qPrime ≤ Msize, qPrime++,
    k = 2 q + s;
    m = 2 qPrime + s;
    If[k + m < n - 4, M[[q, qPrime]] =
      -1 / 2 * ((n - 4) kappa[n, s] / (2 (n - 1))) ^ 2 * Sum[LAnswer[n, k - 2, q - 1][[j]] *
        ((n - 2 s - 2 i - 2 j + 6) / (n + 3 - i - j) * linearizedVectorPrime[n, m - 2, qPrime -
          1][[i]] - (n - 4) * linearizedVector[n, m - 2, qPrime - 1][[i]]) *
        Int[n - 1 + 2 s, n + 3 - i - j], {i, 1, qPrime + 3}, {j, 1, q + 2}],
      M[[q, qPrime]] = (n - 4) / 2 * ((n - 4) kappa[n, s] / (2 (n - 1))) ^ 2 *
        LAnswer[n, k - 2, q - 1][[q + 2]] *
        linearizedVector[n, m - 2, qPrime - 1][[qPrime + 3]]];];];
For[q = 1, q ≤ Msize, q++,
  For[qPrime = 1, qPrime ≤ Msize, qPrime++,
    k = 2 q + s;
    m = 2 qPrime + s;
    If[k + m < n - 4, MSymm[[q, qPrime]] = (M[[q, qPrime]] + M[[qPrime, q]]) / 2,
      MSymm[[q, qPrime]] = 10^10 (M[[q, qPrime]] + M[[qPrime, q]]) / 2];];];
MSymm] (* // MatrixForm *)

```

```
Math[n_, s_] := Simplify[Math1[n, s] + Math2[n, s] + Math3[n, s]];
```

```

In[ ]:= (** Checking the positive definiteness **)
For[n = 12, n ≤ 35, n++,
  For[s = 2, s ≤ Floor[(n - 4) / 2] - 2, s++,
    Print["{n,s}=", {n, s}, ": " PositiveDefiniteMatrixQ[Math[n, s]]]]]

{n,s}={12, 2}: True
{n,s}={13, 2}: True
{n,s}={14, 2}: True
{n,s}={14, 3}: True
{n,s}={15, 2}: True
{n,s}={15, 3}: True
{n,s}={16, 2}: True
{n,s}={16, 3}: True
{n,s}={16, 4}: True
{n,s}={17, 2}: True
{n,s}={17, 3}: True
{n,s}={17, 4}: True
{n,s}={18, 2}: True
{n,s}={18, 3}: True
{n,s}={18, 4}: True
{n,s}={18, 5}: True
{n,s}={19, 2}: True

```

$\{n, s\} = \{19, 3\} : \text{True}$   
 $\{n, s\} = \{19, 4\} : \text{True}$   
 $\{n, s\} = \{19, 5\} : \text{True}$   
 $\{n, s\} = \{20, 2\} : \text{True}$   
 $\{n, s\} = \{20, 3\} : \text{True}$   
 $\{n, s\} = \{20, 4\} : \text{True}$   
 $\{n, s\} = \{20, 5\} : \text{True}$   
 $\{n, s\} = \{20, 6\} : \text{True}$   
 $\{n, s\} = \{21, 2\} : \text{True}$   
 $\{n, s\} = \{21, 3\} : \text{True}$   
 $\{n, s\} = \{21, 4\} : \text{True}$   
 $\{n, s\} = \{21, 5\} : \text{True}$   
 $\{n, s\} = \{21, 6\} : \text{True}$   
 $\{n, s\} = \{22, 2\} : \text{True}$   
 $\{n, s\} = \{22, 3\} : \text{True}$   
 $\{n, s\} = \{22, 4\} : \text{True}$   
 $\{n, s\} = \{22, 5\} : \text{True}$   
 $\{n, s\} = \{22, 6\} : \text{True}$   
 $\{n, s\} = \{22, 7\} : \text{True}$   
 $\{n, s\} = \{23, 2\} : \text{True}$   
 $\{n, s\} = \{23, 3\} : \text{True}$   
 $\{n, s\} = \{23, 4\} : \text{True}$   
 $\{n, s\} = \{23, 5\} : \text{True}$   
 $\{n, s\} = \{23, 6\} : \text{True}$   
 $\{n, s\} = \{23, 7\} : \text{True}$   
 $\{n, s\} = \{24, 2\} : \text{True}$   
 $\{n, s\} = \{24, 3\} : \text{True}$   
 $\{n, s\} = \{24, 4\} : \text{True}$   
 $\{n, s\} = \{24, 5\} : \text{True}$   
 $\{n, s\} = \{24, 6\} : \text{True}$   
 $\{n, s\} = \{24, 7\} : \text{True}$   
 $\{n, s\} = \{24, 8\} : \text{True}$   
 $\{n, s\} = \{25, 2\} : \text{True}$   
 $\{n, s\} = \{25, 3\} : \text{True}$   
 $\{n, s\} = \{25, 4\} : \text{True}$   
 $\{n, s\} = \{25, 5\} : \text{True}$   
 $\{n, s\} = \{25, 6\} : \text{True}$   
 $\{n, s\} = \{25, 7\} : \text{True}$   
 $\{n, s\} = \{25, 8\} : \text{True}$

```

{n,s}={26, 2}: True
{n,s}={26, 3}: True
{n,s}={26, 4}: True
{n,s}={26, 5}: True
{n,s}={26, 6}: True
{n,s}={26, 7}: True
{n,s}={26, 8}: True
{n,s}={26, 9}: True
{n,s}={27, 2}: True
{n,s}={27, 3}: True
{n,s}={27, 4}: True
{n,s}={27, 5}: True
{n,s}={27, 6}: True
{n,s}={27, 7}: True
{n,s}={27, 8}: True
{n,s}={27, 9}: True
{n,s}={28, 2}: True
{n,s}={28, 3}: True
{n,s}={28, 4}: True
{n,s}={28, 5}: True
{n,s}={28, 6}: True
{n,s}={28, 7}: True
{n,s}={28, 8}: True
{n,s}={28, 9}: True
{n,s}={28, 10}: True
{n,s}={29, 2}: True
{n,s}={29, 3}: True
{n,s}={29, 4}: True
{n,s}={29, 5}: True
{n,s}={29, 6}: True
{n,s}={29, 7}: True
{n,s}={29, 8}: True
{n,s}={29, 9}: True
{n,s}={29, 10}: True
{n,s}={30, 2}: True
{n,s}={30, 3}: True
{n,s}={30, 4}: True
{n,s}={30, 5}: True
{n,s}={30, 6}: True

```

```

{n,s}={30, 7}: True
{n,s}={30, 8}: True
{n,s}={30, 9}: True
{n,s}={30, 10}: True
{n,s}={30, 11}: True
{n,s}={31, 2}: True
{n,s}={31, 3}: True
{n,s}={31, 4}: True
{n,s}={31, 5}: True
{n,s}={31, 6}: True
{n,s}={31, 7}: True
{n,s}={31, 8}: True
{n,s}={31, 9}: True
{n,s}={31, 10}: True
{n,s}={31, 11}: True
{n,s}={32, 2}: True
{n,s}={32, 3}: True
{n,s}={32, 4}: True
{n,s}={32, 5}: True
{n,s}={32, 6}: True
{n,s}={32, 7}: True
{n,s}={32, 8}: True
{n,s}={32, 9}: True
{n,s}={32, 10}: True
{n,s}={32, 11}: True
{n,s}={32, 12}: True
{n,s}={33, 2}: False
{n,s}={33, 3}: True
{n,s}={33, 4}: True
{n,s}={33, 5}: True
{n,s}={33, 6}: True
{n,s}={33, 7}: True
{n,s}={33, 8}: True
{n,s}={33, 9}: True
{n,s}={33, 10}: True
{n,s}={33, 11}: True
{n,s}={33, 12}: True
{n,s}={34, 2}: False
{n,s}={34, 3}: True

```

```
{n,s}={34, 4}: True
{n,s}={34, 5}: True
{n,s}={34, 6}: True
{n,s}={34, 7}: True
{n,s}={34, 8}: True
{n,s}={34, 9}: True
{n,s}={34, 10}: True
{n,s}={34, 11}: True
{n,s}={34, 12}: True
{n,s}={34, 13}: True
{n,s}={35, 2}: False
{n,s}={35, 3}: True
{n,s}={35, 4}: True
{n,s}={35, 5}: True
{n,s}={35, 6}: True
{n,s}={35, 7}: True
{n,s}={35, 8}: True
{n,s}={35, 9}: True
{n,s}={35, 10}: True
{n,s}={35, 11}: True
{n,s}={35, 12}: True
{n,s}={35, 13}: True
```
