# Supplementary material for: Compactness and non-compactness theorems of the fourth- and sixth-order constant $Q$-curvature problems
Source: arXiv:2502.14237 ancillary file (2025-09-19)
Supplement: Supplementary file 2 [file Lemmas_B.11_B.12.pdf]

```

In[*]:= (* Integrals and coefficients *)
Int[i_, j_] := Integrate[t^i / (1 + t^2)^j, {t, 0, Infinity}]
Int2[i_, j_] := Integrate[(1 - t^2) t^i / (1 + t^2)^j, {t, 0, Infinity}]
c1[n_, k_, m_] := (k + m) (n^3 - (k + m + 2) n^2 + (6 (k + m) - 4) n - 4 (k + m) + 8);
c2[n_, k_, m_] := 2 (n - 1) (k + m) (n + k + m - 2) k m;

(* Case 1: Estimate of $J_1$ with $H = D$ *)
(** Definition of the matrix **)
MatD[n_, s_] := Module[{d, Msize, q, qPrime, k, m, lambdaq, lambdaqPrime, M},
  d = Floor[(n - 4) / 2];
  Msize = Floor[(d - s) / 2] + 1;
  M = ConstantArray[0, {Msize, Msize}];
  For[q = 0, q ≤ Msize - 1, q++,
    For[qPrime = 0, qPrime ≤ Msize - 1, qPrime++,
      k = 2 q + s;
      m = 2 qPrime + s;
      lambdaq = -q (n + 2 q + 2 s - 2);
      lambdaqPrime = -qPrime (n + 2 qPrime + 2 s - 2);
      If[k + m < n - 4, M[[q + 1, qPrime + 1]] = 1 / (n - k - m - 4) * Int[n + k + m - 3, n - 2]
        ((8 (n - 1) (n - 3) (k + m)) / ((n - 2) (n + k + m - 4)) * lambdaq * lambdaqPrime + 1 / 8 *
          c1[n, k, m] (2 (lambdaq + lambdaqPrime) + (n + k + m - 2) (k + m)) - c2[n, k, m]),
        M[[q + 1, qPrime + 1]] = 10^10 / (2 (n - 3)) *
          ((8 (n - 1) (n - 3) (k + m)) / ((n - 2) (n + k + m - 4)) * lambdaq * lambdaqPrime +
            1 / 8 * c1[n, k, m] (2 (lambdaq + lambdaqPrime) + (n + k + m - 2) (k + m)) -
            c2[n, k, m])];];];
  M] (* // MatrixForm *)

In[*]:= (** Checking the positive definiteness **)
For[n = 8, n ≤ 30, n++,
  For[s = 2, s ≤ Floor[(n - 4) / 2], s++,
    Print["{n,s}=", {n, s}, ": " PositiveDefiniteMatrixQ[MatD[n, s]]]]]

{n,s}={8, 2}: True
{n,s}={9, 2}: True
{n,s}={10, 2}: True
{n,s}={10, 3}: True
{n,s}={11, 2}: True
{n,s}={11, 3}: True
{n,s}={12, 2}: True
{n,s}={12, 3}: True
{n,s}={12, 4}: True
{n,s}={13, 2}: True
{n,s}={13, 3}: True
{n,s}={13, 4}: True
{n,s}={14, 2}: True

```

$\{n, s\} = \{14, 3\} : \text{True}$   
 $\{n, s\} = \{14, 4\} : \text{True}$   
 $\{n, s\} = \{14, 5\} : \text{True}$   
 $\{n, s\} = \{15, 2\} : \text{True}$   
 $\{n, s\} = \{15, 3\} : \text{True}$   
 $\{n, s\} = \{15, 4\} : \text{True}$   
 $\{n, s\} = \{15, 5\} : \text{True}$   
 $\{n, s\} = \{16, 2\} : \text{True}$   
 $\{n, s\} = \{16, 3\} : \text{True}$   
 $\{n, s\} = \{16, 4\} : \text{True}$   
 $\{n, s\} = \{16, 5\} : \text{True}$   
 $\{n, s\} = \{16, 6\} : \text{True}$   
 $\{n, s\} = \{17, 2\} : \text{True}$   
 $\{n, s\} = \{17, 3\} : \text{True}$   
 $\{n, s\} = \{17, 4\} : \text{True}$   
 $\{n, s\} = \{17, 5\} : \text{True}$   
 $\{n, s\} = \{17, 6\} : \text{True}$   
 $\{n, s\} = \{18, 2\} : \text{True}$   
 $\{n, s\} = \{18, 3\} : \text{True}$   
 $\{n, s\} = \{18, 4\} : \text{True}$   
 $\{n, s\} = \{18, 5\} : \text{True}$   
 $\{n, s\} = \{18, 6\} : \text{True}$   
 $\{n, s\} = \{18, 7\} : \text{True}$   
 $\{n, s\} = \{19, 2\} : \text{True}$   
 $\{n, s\} = \{19, 3\} : \text{True}$   
 $\{n, s\} = \{19, 4\} : \text{True}$   
 $\{n, s\} = \{19, 5\} : \text{True}$   
 $\{n, s\} = \{19, 6\} : \text{True}$   
 $\{n, s\} = \{19, 7\} : \text{True}$   
 $\{n, s\} = \{20, 2\} : \text{True}$   
 $\{n, s\} = \{20, 3\} : \text{True}$   
 $\{n, s\} = \{20, 4\} : \text{True}$   
 $\{n, s\} = \{20, 5\} : \text{True}$   
 $\{n, s\} = \{20, 6\} : \text{True}$   
 $\{n, s\} = \{20, 7\} : \text{True}$   
 $\{n, s\} = \{20, 8\} : \text{True}$   
 $\{n, s\} = \{21, 2\} : \text{True}$   
 $\{n, s\} = \{21, 3\} : \text{True}$   
 $\{n, s\} = \{21, 4\} : \text{True}$

```

{n,s}={21, 5}: True
{n,s}={21, 6}: True
{n,s}={21, 7}: True
{n,s}={21, 8}: True
{n,s}={22, 2}: True
{n,s}={22, 3}: True
{n,s}={22, 4}: True
{n,s}={22, 5}: True
{n,s}={22, 6}: True
{n,s}={22, 7}: True
{n,s}={22, 8}: True
{n,s}={22, 9}: True
{n,s}={23, 2}: True
{n,s}={23, 3}: True
{n,s}={23, 4}: True
{n,s}={23, 5}: True
{n,s}={23, 6}: True
{n,s}={23, 7}: True
{n,s}={23, 8}: True
{n,s}={23, 9}: True
{n,s}={24, 2}: True
{n,s}={24, 3}: True
{n,s}={24, 4}: True
{n,s}={24, 5}: True
{n,s}={24, 6}: True
{n,s}={24, 7}: True
{n,s}={24, 8}: True
{n,s}={24, 9}: True
{n,s}={24, 10}: True
{n,s}={25, 2}: False
{n,s}={25, 3}: True
{n,s}={25, 4}: True
{n,s}={25, 5}: True
{n,s}={25, 6}: True
{n,s}={25, 7}: True
{n,s}={25, 8}: True
{n,s}={25, 9}: True
{n,s}={25, 10}: True
{n,s}={26, 2}: False

```

```
{n,s}={26, 3}: True
{n,s}={26, 4}: True
{n,s}={26, 5}: True
{n,s}={26, 6}: True
{n,s}={26, 7}: True
{n,s}={26, 8}: True
{n,s}={26, 9}: True
{n,s}={26, 10}: True
{n,s}={26, 11}: True
{n,s}={27, 2}: False
{n,s}={27, 3}: True
{n,s}={27, 4}: True
{n,s}={27, 5}: True
{n,s}={27, 6}: True
{n,s}={27, 7}: True
{n,s}={27, 8}: True
{n,s}={27, 9}: True
{n,s}={27, 10}: True
{n,s}={27, 11}: True
{n,s}={28, 2}: False
{n,s}={28, 3}: True
{n,s}={28, 4}: True
{n,s}={28, 5}: True
{n,s}={28, 6}: True
{n,s}={28, 7}: True
{n,s}={28, 8}: True
{n,s}={28, 9}: True
{n,s}={28, 10}: True
{n,s}={28, 11}: True
{n,s}={28, 12}: True
{n,s}={29, 2}: False
{n,s}={29, 3}: True
{n,s}={29, 4}: True
{n,s}={29, 5}: True
{n,s}={29, 6}: True
{n,s}={29, 7}: True
{n,s}={29, 8}: True
{n,s}={29, 9}: True
{n,s}={29, 10}: True
```

```

{n,s}={29, 11}: True
{n,s}={29, 12}: True
{n,s}={30, 2}: False
{n,s}={30, 3}: True
{n,s}={30, 4}: True
{n,s}={30, 5}: True
{n,s}={30, 6}: True
{n,s}={30, 7}: True
{n,s}={30, 8}: True
{n,s}={30, 9}: True
{n,s}={30, 10}: True
{n,s}={30, 11}: True
{n,s}={30, 12}: True
{n,s}={30, 13}: True

```

```

In[*]:= (* Case 2: Estimate of  $J_1$  with  $H = W$  *)
(** Definition of the matrix **)
MatW[n_, s_] := Module[{d, Msize, q, qPrime, k, m, lambdaq, lambdaqPrime, M},
  d = Floor[(n - 4) / 2];
  Msize = Floor[(d - s) / 2];
  M = ConstantArray[0, {Msize, Msize}];
  For[q = 1, q ≤ Msize, q++,
    For[qPrime = 1, qPrime ≤ Msize, qPrime++,
      k = 2 q + s;
      m = 2 qPrime + s;
      lambdaq = -1 / 2 (s + 2 q) (n + 2 q + s - 2);
      lambdaqPrime = -1 / 2 (s + 2 qPrime) (n + 2 qPrime + s - 2);
      If[k + m < n - 4, M[[q, qPrime]] = 1 / (n - k - m - 4) *
        Int[n + k + m - 3, n - 2] ((4 (n - 1) (n - 3) (k + m)) / ((n - 2) (n + k + m - 4)) *
          (4 s (n + s + 1) lambdaq * lambdaqPrime + k m s^2 (n + s)^2) +
          2 s (n + s + 1) (1 / 8 * c1[n, k, m] (2 (lambdaq + lambdaqPrime) +
            (n + k + m - 2) (k + m)) - c2[n, k, m])), M[[q, qPrime]] =
          10^10 / (2 (n - 3)) ((4 (n - 1) (n - 3) (k + m)) / ((n - 2) (n + k + m - 4)) *
            (4 s (n + s + 1) lambdaq * lambdaqPrime + k m s^2 (n + s)^2) +
            2 s (n + s + 1) (1 / 8 * c1[n, k, m] (2 (lambdaq + lambdaqPrime) +
              (n + k + m - 2) (k + m)) - c2[n, k, m]))];];];
  M] (* // MatrixForm *)

In[*]:= (** Checking the positive definiteness **)
For[n = 8, n ≤ 30, n++,
  For[s = 1, s ≤ Floor[(n - 4) / 2] - 2, s++,
    Print["{n,s}=", {n, s}, ": " PositiveDefiniteMatrixQ[MatW[n, s]]]]]

{n,s}={10, 1}: True
{n,s}={11, 1}: True

```

$\{n, s\} = \{12, 1\} : \text{True}$   
 $\{n, s\} = \{12, 2\} : \text{True}$   
 $\{n, s\} = \{13, 1\} : \text{True}$   
 $\{n, s\} = \{13, 2\} : \text{True}$   
 $\{n, s\} = \{14, 1\} : \text{True}$   
 $\{n, s\} = \{14, 2\} : \text{True}$   
 $\{n, s\} = \{14, 3\} : \text{True}$   
 $\{n, s\} = \{15, 1\} : \text{True}$   
 $\{n, s\} = \{15, 2\} : \text{True}$   
 $\{n, s\} = \{15, 3\} : \text{True}$   
 $\{n, s\} = \{16, 1\} : \text{True}$   
 $\{n, s\} = \{16, 2\} : \text{True}$   
 $\{n, s\} = \{16, 3\} : \text{True}$   
 $\{n, s\} = \{16, 4\} : \text{True}$   
 $\{n, s\} = \{17, 1\} : \text{True}$   
 $\{n, s\} = \{17, 2\} : \text{True}$   
 $\{n, s\} = \{17, 3\} : \text{True}$   
 $\{n, s\} = \{17, 4\} : \text{True}$   
 $\{n, s\} = \{18, 1\} : \text{True}$   
 $\{n, s\} = \{18, 2\} : \text{True}$   
 $\{n, s\} = \{18, 3\} : \text{True}$   
 $\{n, s\} = \{18, 4\} : \text{True}$   
 $\{n, s\} = \{18, 5\} : \text{True}$   
 $\{n, s\} = \{19, 1\} : \text{True}$   
 $\{n, s\} = \{19, 2\} : \text{True}$   
 $\{n, s\} = \{19, 3\} : \text{True}$   
 $\{n, s\} = \{19, 4\} : \text{True}$   
 $\{n, s\} = \{19, 5\} : \text{True}$   
 $\{n, s\} = \{20, 1\} : \text{True}$   
 $\{n, s\} = \{20, 2\} : \text{True}$   
 $\{n, s\} = \{20, 3\} : \text{True}$   
 $\{n, s\} = \{20, 4\} : \text{True}$   
 $\{n, s\} = \{20, 5\} : \text{True}$   
 $\{n, s\} = \{20, 6\} : \text{True}$   
 $\{n, s\} = \{21, 1\} : \text{True}$   
 $\{n, s\} = \{21, 2\} : \text{True}$   
 $\{n, s\} = \{21, 3\} : \text{True}$   
 $\{n, s\} = \{21, 4\} : \text{True}$   
 $\{n, s\} = \{21, 5\} : \text{True}$

```

{n,s}={21, 6}: True
{n,s}={22, 1}: True
{n,s}={22, 2}: True
{n,s}={22, 3}: True
{n,s}={22, 4}: True
{n,s}={22, 5}: True
{n,s}={22, 6}: True
{n,s}={22, 7}: True
{n,s}={23, 1}: True
{n,s}={23, 2}: True
{n,s}={23, 3}: True
{n,s}={23, 4}: True
{n,s}={23, 5}: True
{n,s}={23, 6}: True
{n,s}={23, 7}: True
{n,s}={24, 1}: True
{n,s}={24, 2}: True
{n,s}={24, 3}: True
{n,s}={24, 4}: True
{n,s}={24, 5}: True
{n,s}={24, 6}: True
{n,s}={24, 7}: True
{n,s}={24, 8}: True
{n,s}={25, 1}: True
{n,s}={25, 2}: True
{n,s}={25, 3}: True
{n,s}={25, 4}: True
{n,s}={25, 5}: True
{n,s}={25, 6}: True
{n,s}={25, 7}: True
{n,s}={25, 8}: True
{n,s}={26, 1}: True
{n,s}={26, 2}: True
{n,s}={26, 3}: True
{n,s}={26, 4}: True
{n,s}={26, 5}: True
{n,s}={26, 6}: True
{n,s}={26, 7}: True
{n,s}={26, 8}: True

```

```
{n,s}={26, 9}: True
{n,s}={27, 1}: True
{n,s}={27, 2}: True
{n,s}={27, 3}: True
{n,s}={27, 4}: True
{n,s}={27, 5}: True
{n,s}={27, 6}: True
{n,s}={27, 7}: True
{n,s}={27, 8}: True
{n,s}={27, 9}: True
{n,s}={28, 1}: True
{n,s}={28, 2}: True
{n,s}={28, 3}: True
{n,s}={28, 4}: True
{n,s}={28, 5}: True
{n,s}={28, 6}: True
{n,s}={28, 7}: True
{n,s}={28, 8}: True
{n,s}={28, 9}: True
{n,s}={28, 10}: True
{n,s}={29, 1}: False
{n,s}={29, 2}: True
{n,s}={29, 3}: True
{n,s}={29, 4}: True
{n,s}={29, 5}: True
{n,s}={29, 6}: True
{n,s}={29, 7}: True
{n,s}={29, 8}: True
{n,s}={29, 9}: True
{n,s}={29, 10}: True
{n,s}={30, 1}: False
{n,s}={30, 2}: True
{n,s}={30, 3}: True
{n,s}={30, 4}: True
{n,s}={30, 5}: True
{n,s}={30, 6}: True
{n,s}={30, 7}: True
{n,s}={30, 8}: True
{n,s}={30, 9}: True
```



```
{n,s}={30, 10}: True
```

```
{n,s}={30, 11}: True
```
